# Supplementary material for: Feature-based factorized Bilinear Similarity Model for Cold-Start Top-n Item Recommendation
Source: arXiv:1904.11799 source file (2019-04-22)
Supplement: Supplementary file 1 [file supp.tex]

%!TEX root = bilinear.tex
\setcounter{page}{1}
\setcounter{table}{1}
\setcounter{section}{0}

\begin{center}
{\large Factorized Bilinear Similiarty for Cold-Start Item Recommendation }\\
Supplementary Materials\\
\quad\\
Mohit Sharma, Jiayu Zhou, Junling Hu, George Karypis
\end{center}

\section{Computation Efficiency of FBSM$_{bpr}$}
In FBSM$_{bpr}$, we used stochastic gradient descent to update the variables.
The key to FBSM$_{pbr}$ is to efficiently compute the relative rank
$\tilde{r}_{u,ij}$ and the two gradients $\nabla_{\bm{d}} \tilde{r}_{u,ij}$, $
\nabla_{\bm{v}_{p}} \tilde{r}_{u,ij}$ in Eq.~(\ref{dUpdBPREq}) and
Eq.~(\ref{vUpdBPREq}). In this section we show in details how the gradients are derived
and how these components can be efficiently computed.

In order to efficient compute these components, we will need to pre-compute 
some components and cache them during the optimization. 
Firstly we need to compute this global variable once:
\begin{equation*}
  F_q = \sum_{\substack{ q \in \mathcal{R}_u^+}}\bm{f}_q, 
\end{equation*}
And also compute the following variables each time we compute gradient: 
\begin{equation*}
  Z_q = \sum_{\substack{l=1}}^{n_F}\bm{v}_lF_{ql},\\ 
  \Delta_{ij} = \sum_{l=1}^{n_F} (f_{il}-f_{jl}), \\ 
  C_{\Delta_{ij}} = \sum_{l=1}^{n_F} (f_{il}-f_{jl})\bm{v}_l, \\ 
  C_i = \sum_{l=1}^{n_F}f_{il}\bm{v}_l, \\ 
  C_j = \sum_{l=1}^{n_F}f_{jl}\bm{v}_l 
\end{equation*}

\subsection{Computation of Relative Rank}
\begin{equation} \label{relRankExpanded}
\begin{split}
  \tilde{r}_{u,ij} &= r_{u,i} - r_{u,j} \\
  &= \bm{f}_i^T\diag(\bm{d})(F_q-\bm{f}_i) + \sum_{k=1}^{n_F}f_{ik}\bm{v}_k^T\sum_{\substack{p=1 ,\\ p \neq k}}^{n_F} \bm{v}_p(F_{qp}-f_{ip}) - \left\{ \bm{f}_j^T\diag(\bm{d})F_q + \sum_{k=1}^{n_F}f_{jk}\bm{v}_k^T\sum_{\substack{p=1 ,\\ p \neq k}}^{n_F} \bm{v}_pF_{qp}\ \right\}\\
  %&= (f_i-f_j)^Tdiag(d)F_q - f_i^Tdiag(d)f_i + \sum_{k=1}^{n_F}(f_{ik}-f_{jk})v_k^T\sum_{\substack{p=1 ,\\ p \neq k}}^{n_F} v_pF_{qp} - \sum_{k=1}^{n_F}f_{ik}v_k^T\sum_{\substack{p=1 ,\\ p \neq k}}^{n_F} v_pf_{ip} \\
  %&= \Delta_{ij}^Tdiag(d)F_q - f_i^Tdiag(d)f_i + \sum_{k=1}^{n_F}\Delta_{ij,k}v_k^T\sum_{\substack{p=1 ,\\ p \neq k}}^{n_F} v_pF_{qp} - \sum_{k=1}^{n_F}f_{ik}v_k^T\sum_{\substack{p=1 ,\\ p \neq k}}^{n_F} v_pf_{ip} \\
  &= \Delta_{ij}^T\diag(\bm{d})F_q - \bm{f}_i^T\diag(\bm{d})\bm{f}_i + \sum_{k=1}^{n_F}\Delta_{ij,k}\bm{v}_k^T(Z_q - \bm{v}_kF_{qk}) - \sum_{k=1}^{n_F}f_{ik}\bm{v}_k^T(C_i-\bm{v}_kf_{ik}) \\
\end{split}
\end{equation}

\subsection{Computation of Gradient}

\subsubsection{The diagnoal component. } 

\begin{equation}  \label{diagGradBPREq}
  \frac{\partial}{\partial d_{c}} \tilde{r}_{u,ij} = \Delta_{ij,c}F_{qc}-f_{i,c}^2 
\end{equation}

\subsubsection{The low-rank component. }

\begin{equation}
  \begin{split}
    \nabla_{\bm{v}_{p}} \tilde{r}_{u,ij} 
     %&= \nabla_{\bm{v}_{p}}\left\{\sum_{k=1}^{n_F}\Delta_{ij,k}v_k^T\sum_{\substack{l=1 ,\\ l \neq k}}^{n_F} v_lF_{ql} - \sum_{k=1}^{n_F}f_{ik}v_k^T\sum_{\substack{l=1 ,\\ l \neq k}}^{n_F} v_lf_{il} \right\}  \\ 
     % &= \frac{\partial}{\partial v_{p}}\left\{\Delta_{ij,p}v_p^T\sum_{\substack{l=1 ,\\ l \neq p}}^{n_F} v_lF_{ql} + \sum_{\substack{k=1, \\ k \neq p}}^{n_F}\Delta_{ij,k}v_k^Tv_pF_{qp} - f_{ip}v_p^T\sum_{\substack{l=1 ,\\ l \neq p}}^{n_F} v_lf_{il}  - \sum_{\substack{k=1, \\ k \neq p}}^{n_F}f_{ik}v_k^Tv_pf_{ip} \right\}  \\ 
     &= \nabla_{\bm{v}_{p}}\left\{\Delta_{ij,p}\bm{v}_p^T\sum_{\substack{l=1 ,\\ l \neq p}}^{n_F} \bm{v}_lF_{ql} + \bm{v}_pF_{qp} \sum_{\substack{k=1, \\ k \neq p}}^{n_F}\Delta_{ij,k}\bm{v}_k^T- f_{ip}\bm{v}_p^T\sum_{\substack{l=1 ,\\ l \neq p}}^{n_F} \bm{v}_lf_{il}  - \bm{v}_pf_{ip} \sum_{\substack{k=1, \\ k \neq p}}^{n_F}f_{ik}\bm{v}_k^T\right\}  \\ 
     &= \Delta_{ij,p}\sum_{\substack{l=1 ,\\ l \neq p}}^{n_F} \bm{v}_lF_{ql} + F_{qp} \sum_{\substack{k=1, \\ k \neq p}}^{n_F}\Delta_{ij,k}\bm{v}_k- f_{ip}\sum_{\substack{l=1 ,\\ l \neq p}}^{n_F} \bm{v}_lf_{il} - f_{ip} \sum_{\substack{k=1, \\ k \neq p}}^{n_F}f_{ik}\bm{v}_k  \\ 
     %&= \Delta_{ij,p}\sum_{\substack{l=1 ,\\ l \neq p}}^{n_F} v_lF_{ql} + F_{qp} \sum_{\substack{k=1, \\ k \neq p}}^{n_F}\Delta_{ij,k}v_k- 2f_{ip}\sum_{\substack{l=1 ,\\ l \neq p}}^{n_F} v_lf_{il} \\ 
     %&= \Delta_{ij,p}(Z_q - v_pF_{qp}) + F_{qp} \sum_{\substack{k=1, \\ k \neq p}}^{n_F}\Delta_{ij,k}v_k- 2f_{ip}(C_i - v_pf_{ip}) \\ 
     &= \Delta_{ij,p}(Z_q - \bm{v}_pF_{qp}) + F_{qp}(C_{\Delta_{ij}}-\Delta_{ij,p}\bm{v}_p) - 2f_{ip}(C_i - \bm{v}_pf_{ip}) \\ 
  \end{split}
\end{equation}
